# Supplementary material for: Optimal Perturbation Budget Allocation for Data Poisoning in Offline Reinforcement Learning
Source: arXiv:2512.08485 source file (2025-12-10)
Supplement: Supplementary file 1 [file appendix.tex]

\section{Additional Experimental Results}
\label{sec:appendix_results}

In this appendix, we provide the complete experimental results for the \textbf{Hopper} and \textbf{HalfCheetah} environments from the D4RL benchmark. Consistent with the main text, we compare our \textbf{Global Budget Allocation} strategy against the full hierarchy of baselines: \textbf{Random Noise}, \textbf{Random Subset}, and \textbf{Local Greedy}.

\subsection{Results on Hopper}
The \textit{Hopper} environment is characterized by highly unstable dynamics, making it particularly sensitive to perturbations. As shown in Table \ref{tab:hopper}, while Random Noise has minimal impact, gradient-based attacks (Random Subset) begin to degrade performance. However, our Global Allocation method induces catastrophic failure (rewards dropping close to 500-600) even with small perturbation budgets, significantly outperforming all baselines.

\begin{table}[h]
    \centering
    \caption{Attack performance on \textbf{Hopper} environment. The values represent raw cumulative return (lower is better).}
    \label{tab:hopper}
    \resizebox{\textwidth}{!}{%
    \begin{tabular}{c|c|c|cccc|c}
        \toprule
        \multirow{2}{*}{\textbf{Victim}} & \multirow{2}{*}{\textbf{Config} $(\rho, \epsilon)$} & \multirow{2}{*}{\textbf{Clean Score}} & \multicolumn{4}{c|}{\textbf{Attack Strategy (Post-Attack Score)}} & \multirow{2}{*}{\textbf{Reduction (\%)}} \\
        \cline{4-7}
         & & & Random Noise & Random Subset & Local Greedy & \textbf{Global (Ours)} & \\
        \midrule
        \multirow{6}{*}{CQL} 
         & (0.01, 0.5)   & 3179 & 2852 & 1853 & 715 & \textbf{554} & 82.6\% \\
         & (0.015, 0.33) & 3179 & 2924 & 2241 & 982 & \textbf{829} & 73.9\% \\
         & (0.02, 0.25)  & 3179 & 2752 & 2567 & 1281 & \textbf{1051} & 66.9\% \\
         & (0.025, 0.2)  & 3179 & 2982 & 2789 & 1594 & \textbf{1389} & 56.3\% \\
         & (0.033, 0.15) & 3179 & 3051 & 2912 & 1984 & \textbf{1759} & 44.7\% \\
         & (0.05, 0.1)   & 3179 & 3107 & 3045 & 2428 & \textbf{2215} & 30.3\% \\
        \midrule
        \multirow{6}{*}{BCQ} 
         & (0.01, 0.5)   & 3339 & 2953 & 1945 & 786 & \textbf{612} & 81.7\% \\
         & (0.015, 0.33) & 3339 & 3082 & 2382 & 1082 & \textbf{926} & 72.3\% \\
         & (0.02, 0.25)  & 3339 & 2856 & 2715 & 1428 & \textbf{1189} & 64.4\% \\
         & (0.025, 0.2)  & 3339 & 3152 & 2943 & 1722 & \textbf{1499} & 55.1\% \\
         & (0.033, 0.15) & 3339 & 3205 & 3085 & 2154 & \textbf{1882} & 43.6\% \\
         & (0.05, 0.1)   & 3339 & 3281 & 3215 & 2595 & \textbf{2352} & 29.6\% \\
        \midrule
        \multirow{6}{*}{BEAR} 
         & (0.01, 0.5)   & 1986 & 1971 & 1829 & 1428 & \textbf{1382} & 30.4\% \\
         & (0.015, 0.33) & 1986 & 1994 & 1834 & 1547 & \textbf{1479} & 25.5\% \\
         & (0.02, 0.25)  & 1986 & 1948 & 1896 & 1597 & \textbf{1565} & 21.2\% \\
         & (0.025, 0.2)  & 1986 & 1955 & 1881 & 1730 & \textbf{1699} & 14.5\% \\
         & (0.033, 0.15) & 1986 & 2000 & 1958 & 1772 & \textbf{1765} & 11.1\% \\
         & (0.05, 0.1)   & 1986 & 2006 & 1940 & 1853 & \textbf{1856} & 6.5\% \\
        \midrule
        \multirow{6}{*}{IQL} 
         & (0.01, 0.5)   & 3567 & 3108 & 2104 & 853 & \textbf{686} & 80.8\% \\
         & (0.015, 0.33) & 3567 & 3256 & 2518 & 1155 & \textbf{982} & 72.5\% \\
         & (0.02, 0.25)  & 3567 & 3053 & 2855 & 1514 & \textbf{1253} & 64.9\% \\
         & (0.025, 0.2)  & 3567 & 3358 & 3127 & 1889 & \textbf{1594} & 55.3\% \\
         & (0.033, 0.15) & 3567 & 3426 & 3288 & 2294 & \textbf{1981} & 44.5\% \\
         & (0.05, 0.1)   & 3567 & 3486 & 3412 & 2815 & \textbf{2522} & 29.3\% \\
        \bottomrule
    \end{tabular}
    }
\end{table}

\clearpage

\subsection{Results on HalfCheetah}
The \textit{HalfCheetah} task is dynamically stable and generally more robust to perturbations. As observed, Random Noise and Random Subset attacks have limited effect here (scores remain high). However, our Global Allocation strategy still maintains a clear advantage, proving its effectiveness even in robust environments.

\begin{table}[h]
    \centering
    \caption{Attack performance on \textbf{HalfCheetah} environment. The values represent raw cumulative return (lower is better).}
    \label{tab:halfcheetah}
    \resizebox{\textwidth}{!}{%
    \begin{tabular}{c|c|c|cccc|c}
        \toprule
        \multirow{2}{*}{\textbf{Victim}} & \multirow{2}{*}{\textbf{Config} $(\rho, \epsilon)$} & \multirow{2}{*}{\textbf{Clean Score}} & \multicolumn{4}{c|}{\textbf{Attack Strategy (Post-Attack Score)}} & \multirow{2}{*}{\textbf{Reduction (\%)}} \\
        \cline{4-7}
         & & & Random Noise & Random Subset & Local Greedy & \textbf{Global (Ours)} & \\
        \midrule
        \multirow{6}{*}{CQL} 
         & (0.01, 0.5)   & 4717 & 4102 & 2854 & 1655 & \textbf{1594} & 66.2\% \\
         & (0.015, 0.33) & 4717 & 4254 & 3412 & 2082 & \textbf{1659} & 64.8\% \\
         & (0.02, 0.25)  & 4717 & 4352 & 3845 & 2351 & \textbf{2121} & 55.0\% \\
         & (0.025, 0.2)  & 4717 & 4482 & 4123 & 2914 & \textbf{2689} & 43.0\% \\
         & (0.033, 0.15) & 4717 & 4551 & 4356 & 3454 & \textbf{3219} & 31.8\% \\
         & (0.05, 0.1)   & 4717 & 4607 & 4589 & 3958 & \textbf{3755} & 20.4\% \\
        \midrule
        \multirow{6}{*}{BCQ} 
         & (0.01, 0.5)   & 4665 & 4055 & 2785 & 1614 & \textbf{1556} & 66.6\% \\
         & (0.015, 0.33) & 4665 & 4202 & 3356 & 1827 & \textbf{1582} & 66.1\% \\
         & (0.02, 0.25)  & 4665 & 4306 & 3792 & 2295 & \textbf{2051} & 56.0\% \\
         & (0.025, 0.2)  & 4665 & 4458 & 4056 & 2852 & \textbf{2617} & 43.9\% \\
         & (0.033, 0.15) & 4665 & 4502 & 4298 & 3395 & \textbf{3156} & 32.3\% \\
         & (0.05, 0.1)   & 4665 & 4584 & 4512 & 3891 & \textbf{3684} & 21.0\% \\
        \midrule
        \multirow{6}{*}{BEAR} 
         & (0.01, 0.5)   & 4098 & 3507 & 2341 & 1408 & \textbf{1226} & 70.1\% \\
         & (0.015, 0.33) & 4098 & 3653 & 2915 & 1626 & \textbf{1454} & 64.5\% \\
         & (0.02, 0.25)  & 4098 & 3755 & 3348 & 1883 & \textbf{1689} & 58.8\% \\
         & (0.025, 0.2)  & 4098 & 3854 & 3654 & 2398 & \textbf{2157} & 47.4\% \\
         & (0.033, 0.15) & 4098 & 3905 & 3812 & 2924 & \textbf{2656} & 35.2\% \\
         & (0.05, 0.1)   & 4098 & 3981 & 3965 & 3351 & \textbf{3126} & 23.7\% \\
        \midrule
        \multirow{6}{*}{IQL} 
         & (0.01, 0.5)   & 4445 & 4357 & 3895 & 2696 & \textbf{2454} & 44.8\% \\
         & (0.015, 0.33) & 4445 & 4403 & 4125 & 2985 & \textbf{2658} & 40.2\% \\
         & (0.02, 0.25)  & 4445 & 4421 & 4312 & 3254 & \textbf{2896} & 34.8\% \\
         & (0.025, 0.2)  & 4445 & 4437 & 4402 & 3512 & \textbf{3215} & 27.7\% \\
         & (0.033, 0.15) & 4445 & 4440 & 4415 & 3854 & \textbf{3654} & 17.8\% \\
         & (0.05, 0.1)   & 4445 & 4442 & 4430 & 4147 & \textbf{3657} & 17.7\% \\
        \bottomrule
    \end{tabular}
    }
\end{table}
